# Supplementary material for: Generalization Error Estimates of Machine Learning Methods for Solving High Dimensional Schr\"odinger Eigenvalue Problems
Source: arXiv:2408.13511 source file (2024-08-24)
Supplement: Supplementary file 1 [file Bounding_Rademacher_complexity_without_L_infinite_norm.tex]

\section{Bounding Rademacher complexity of \texorpdfstring{$\mathcal{G}_{m}^{4, j}$}{}}
\begin{definition}
We define for a set of random variables  $\mathcal{S} = \left\{Z_{j}\right\}_{j=1}^{n}$  independently distributed according to  $\mathcal{P}_{\Omega}$  and a function class  $\mathcal{F}$  the empirical Rademacher complexity
$$\hat{R}_{n}(\mathcal{F}, \mathcal{S}):=\mathbf{E}_{\sigma}\left[\sup _{f \in \mathcal{F}}\left|\frac{1}{n} \sum_{j=1}^{n} \sigma_{j} f\left(Z_{j}\right)\right| \mid Z_{1}, \cdots, Z_{n}\right],$$
where the expectation  $\mathbf{E}_{\sigma}$  is taken with respect to the independent symmetric Bernoulli sequence  $\left\{\sigma_{j}\right\}_{j=1}^{n}$  with  $\sigma_{j} \in\{ \pm 1\}$. The Rademacher complexity of  $\mathcal{F}$  is then defined by  $$R_{n}(\mathcal{F})=\mathbf{E}_{\mathcal{S}}\left[\hat{R}_{n}(\mathcal{F}, \mathcal{S})\right].$$
\end{definition}

\textbf{Bounding  $R_{n}\left(\mathcal{G}_{m}^{4, j}\right) $.} 
Recall that $\{\psi_{j}\}_{j=1}^{k-1}$ are the first $k-1$ orthonormal normalized eigenfunctions. Define for $j = 1, 2, \ldots, k-1,$
$$\mathcal{G}_{m}^{4, j} := \left\{g: \Omega \rightarrow \mathbb{R}\ \left|\ g= \varphi \psi_{j}v_{\theta} \text { where } v_{\theta} \in \widetilde{\mathcal{F}}_{m}\right.\right\}.$$

In order to bound $R_{n}\left(\mathcal{G}_{m}^{4, j}\right) $ without using $L^{\infty}(\Omega)$-norm of $\psi_{j}$, we first introduce a more elaborate Dudley‘s inequality, which can be proved by chaining method.
\begin{theorem}[Dudley's Entropy Integral Bound, {\cite{Dudley1967290},\cite[Theorem 4.6]{Liao2020NotesOR}}] %\label{Dudley's Entropy Integral Bound for empirical Rademacher complexity}
Let  $\mathcal{F}$  be a class of real-valued functions,  $S=\left\{z_{1}, \cdots, z_{m}\right\}$  be a random $i.i.d.$ sample.  Assuming
$$\sup _{f \in \mathcal{F}} \|f\|_{2, \mathcal{S}} := \sup _{f \in \mathcal{F}}\left(\frac{1}{n} \sum_{i=1}^{n} f^{2}\left(z_{i}\right)\right)^{1/2} \leq c.$$
then we have
$$\hat{R}_{n}(\mathcal{F}, S) \leq \inf _{\epsilon \in[0, c / 2]}\left(4 \epsilon + \frac{12}{\sqrt{n}} \int_{\epsilon}^{c / 2} \sqrt{\ln \mathcal{N}\left(\mathcal{F}, \delta,\|\cdot\|_{2, \mathcal{S}}\right)}  d \delta\right)$$    
\end{theorem}

\begin{lemma}\label{lemma: new covering number for Gm4,j}
Assume that the activation function  $\phi$  satisfy Assumption \ref{assumption for activation function}. 
Let $$\mathcal{G}_{m}^{4} := \left\{g: \Omega \rightarrow \mathbb{R}\ \left|\ g= \varphi \psi v_{\theta} \text { where } v_{\theta} \in \widetilde{\mathcal{F}}_{m}\right.\right\}.$$
Then, for any $S=\left\{z_{1}, \cdots, z_{m}\right\}$, the covering number  $\mathcal{N}\left(\delta, \mathcal{G}_{m}^{4},\|\cdot\|_{2, \mathcal{S}}\right)$   satisfies that
\begin{equation} \label{new covering number for Gm4,j}
\begin{aligned}
\mathcal{N}\left(\delta, \mathcal{G}_{m}^{4},\|\cdot\|_{2, \mathcal{S}}\right) \leq \mathcal{M}\left(\delta, \Lambda_{4}, m, d\right)
\end{aligned}
\end{equation}
where the constant  $\Lambda_{4}$  is defined by
\begin{equation} \label{new magnification Lambda4,j for Gm4}
\begin{aligned}
\Lambda_{4} = \|\psi\|_{2, \mathcal{S}}\left(1+\phi_{\max }+2 L \Gamma\right)/d.
\end{aligned}
\end{equation}
\end{lemma}

\begin{proof} 
For any $g_{\theta}, g_{\theta^{\prime}}\in \mathcal{G}_{m}^{4}$,
\begin{equation*} 
\begin{aligned}
\|g_{\theta} - g_{\theta^{\prime}}\|_{2, \mathcal{S}}^{2} & = \frac{1}{n} \sum_{i=1}^{n}\varphi^{2}\left(z_{i}\right) \psi^{2}\left(z_{i}\right)  \left( v_{\theta}\left(z_{i}\right) - v_{\theta^{\prime}}\left(z_{i}\right)\right)^{2} \\
& \leq \frac{1}{d^{2}} \left[\left(1+\phi_{\max }+2 L \Gamma\right) \rho_{\Theta}\left(\theta, \theta^{\prime}\right)\right]^{2} \frac{1}{n} \sum_{i=1}^{n}\left(z_{i}\right) \psi^{2}\left(z_{i}\right)  ,
\end{aligned}
\end{equation*}
where the inequality follows from (\ref{utheta(x)-uthetaprime(x) bounded by rho(theta, thetaprime)}) that 
$$\left|v_{\theta}(x)-v_{\theta^{\prime}}(x)\right| \leq\left(1+\phi_{\max }+2 L \Gamma\right) \rho_{\Theta}\left(\theta, \theta^{\prime}\right)$$
and the bound from Lemma \ref{preliminary bounds for cutoff function varphi(x)} that $0 < \varphi(x) < 1/d$.
Hence, $\|g_{\theta} - g_{\theta^{\prime}}\|_{2, \mathcal{S}} \leq \Lambda_{4} \rho_{\Theta}\left(\theta, \theta^{\prime}\right).$ 
As a consequence,  $\mathcal{N}\left(\delta, \mathcal{G}_{m}^{4},\|\cdot\|_{2, \mathcal{S}}\right) \leq \mathcal{N}\left(\frac{\delta}{\Lambda_{4}}, \Theta, \rho_{\Theta}\right)$. Then the lemma follows from Proposition \ref{Proposition: covering number of parameter space Theta} with  $\delta$  replaced by  $\frac{\delta}{\Lambda_{4}}$.
\end{proof}

The following lemma controls the empirical Rademacher complexity of $\mathcal{G}_{m}^{4}$.
\begin{lemma} \label{control empirical Rademacher complexity of Gm4}
Assume that the activation function  $\phi$  satisfies Assumption \ref{assumption for activation function}. Then
$$\hat{R}_{n}\left(\mathcal{G}_{m}^{4}, S\right) \leq \mathcal{Z}\left(M_{4}, \Lambda_{4}, d\right) \cdot \sqrt{\frac{m}{n}} ,$$
where  $M_{4}=\left(C + \Gamma\phi_{\max}\right) \|\psi\|_{2, \mathcal{S}} /d$  and  $\Lambda_{4}$  is defined in (\ref{new magnification Lambda4,j for Gm4}).
\end{lemma}

\begin{proof}
Thanks to  Assumption \ref{assumption for activation function}, for any $S=\left\{z_{1}, \cdots, z_{m}\right\}$,
\begin{equation*} \label{}
\begin{aligned}
\sup _{g \in \mathcal{G}_{m}^{4}}\|g\|_{2, \mathcal{S}} & \leq \sup_{v \in \widetilde{\mathcal{F}}_{m}} \left(\frac{1}{n} \sum_{i=1}^{n} \varphi^{2}\left(z_{i}\right) \psi^{2} \left(z_{i}\right) v^{2}\left(z_{i}\right)\right)^{1/2} 
\leq \left\|\varphi\right\|_{\infty} \|\psi\|_{2, \mathcal{S}} \sup_{v \in \widetilde{\mathcal{F}}_{m}} \left\| v\right\|_{\infty} 
 \\
& \leq \left(C + \Gamma\phi_{\max}\right) \|\psi\|_{2, \mathcal{S}} /d  =  M_{4} .
\end{aligned}
\end{equation*}
Then the lemma follows from Lemma \ref{lemma: covering number for Gm1}, Theorem \ref{Dudley's Entropy Integral Bound for empirical Rademacher complexity}  with  $\delta=0$, $M=M_{4}$  and the simple fact that  $\sqrt{a+b} \leq \sqrt{a}+\sqrt{b}$  for  $a, b \geq 0$.
\end{proof}

\begin{proposition}
Assume that $\|\psi\|_{L^{2}(\Omega)} = 1$ and that the activation function  $\phi$  satisfies Assumption \ref{assumption for activation function}. Then
\begin{equation*}
\begin{aligned}
R_{n}\left(\mathcal{G}_{m}^{4}\right) & \leq \left[ \left(C + \Gamma\phi_{\max}\right) /d \left( \sqrt{(\ln (18 C\Gamma T)+d \ln (3 W))_{+}} + \sqrt{(d+3) \ln (\left(1+\phi_{\max } + 2 L \Gamma\right)/d + 1) } \right)  \right. 
\\
& \quad  \left. + 4\sqrt{C + \Gamma\phi_{\max}} \right]  \sqrt{\frac{m}{n}}.
\end{aligned}
\end{equation*}
\end{proposition}

\begin{proof}
Let $\mathcal{S} = \left\{Z_{j}\right\}_{j=1}^{n}$ be a set of random variables independently distributed according to  $\mathcal{P}_{\Omega}$. Since $\|\psi\|_{L^{2}(\Omega)} = 1$, by Jensen's ineqoality,
\begin{equation*} \label{expectation bound for |psi|2,mathcalS}
\begin{aligned}
\mathbf{E}_{\mathcal{S}}\|\psi\|_{2, \mathcal{S}} \leq \left[\mathbf{E}_{\mathcal{S}}\left(\frac{1}{n} \sum_{i=1}^{n} \psi^{2}\left(Z_{i}\right)\right) \right]^{1/2} = \left(\mathbf{E}_{\mathcal{S}}\psi^{2}\left(Z_{1}\right) \right)^{1/2} = \|\psi\|_{L^{2}(\Omega)} = 1.
\end{aligned}
\end{equation*}
Thus, $\mathbf{E}_{\mathcal{S}} M_{4} \leq \left( \mathbf{E}_{\mathcal{S}} M_{4}^{2} \right)^{1/2} = \left(C + \Gamma\phi_{\max}\right) /d$ and $\mathbf{E}_{\mathcal{S}} \Lambda_{4} \leq \left(1+\phi_{\max } + 2 L \Gamma\right)/d.$
Recall that
\begin{equation*} 
\begin{aligned}
\mathcal{Z}(M, \Lambda, d) & =  M\left(\sqrt{(\ln (2 C \Lambda) + \ln (3 \Gamma \Lambda)+d \ln (3 W \Lambda)+\ln (3 T \Lambda))_{+}}\right) \\
& \quad +\sqrt{d+3} \int_{0}^{M} \sqrt{(\ln (1 / \varepsilon))_{+}} d \varepsilon \\
& \leq M\left(\sqrt{(\ln (2 C) + \ln (3 \Gamma )+d \ln (3 W )+\ln (3 T ))_{+}} + \sqrt{(d+3)(\ln \Lambda )_{+}} \right) \\
& \quad + \sqrt{d+3} \int_{0}^{\min(1,M)} \sqrt{\ln (1 / \varepsilon)} d \varepsilon,
\end{aligned}
\end{equation*}
where 
\begin{equation*} 
\begin{aligned} 
\int_{0}^{\min(1,M)} \sqrt{\ln (1 / \varepsilon)} d \varepsilon \leq \int_{0}^{\min(1,M)} \sqrt{1 / \varepsilon} d \varepsilon \leq  2\min(1,\sqrt{M}).
\end{aligned}
\end{equation*}
By Cauchy's inequality and Jensen's ineqoality,
\begin{equation*} 
\begin{aligned} 
\mathbf{E}_{\mathcal{S}}\left( M_{4} \sqrt{(\ln \Lambda_{4} )_{+}} \right) &  \leq \left( \mathbf{E}_{\mathcal{S}} M_{4}^{2} \right)^{1/2} \left( \mathbf{E}_{\mathcal{S}} \ln (\Lambda_{4} + 1) \right)^{1/2} \\
&  \leq \left(C + \Gamma\phi_{\max}\right) /d \cdot \sqrt{ \ln (\left(1+\phi_{\max } + 2 L \Gamma\right)/d + 1) },
\end{aligned}
\end{equation*}
and  $\mathbf{E}_{\mathcal{S}}\min(1,\sqrt{M_{4}}) \leq \sqrt{\mathbf{E}_{\mathcal{S}} M_{4}} \leq \sqrt{\left(C + \Gamma\phi_{\max}\right) /d}.$  Combining the estimates above, we obtain
\begin{equation*} 
\begin{aligned}
\mathbf{E}_{\mathcal{S}}\mathcal{Z}(M_{4}, \Lambda_{4}, d) & \leq \sqrt{(\ln (2 C) + \ln (3 \Gamma )+d \ln (3 W )+\ln (3 T ))_{+}} \mathbf{E}_{\mathcal{S}}M_{4}  
\\
& \quad + \sqrt{d+3} \left[\mathbf{E}_{\mathcal{S}}\left(M_{4} \sqrt{(\ln \Lambda )_{+}}\right) + 2\mathbf{E}_{\mathcal{S}} \min(1,\sqrt{M_{4}})\right] \\
& \leq \sqrt{(\ln (18 C\Gamma T)+d \ln (3 W))_{+}}  \left(C + \Gamma\phi_{\max}\right) /d 
\\
& \quad + \sqrt{d+3} \left[ \left(C + \Gamma\phi_{\max}\right)/d \sqrt{ \ln (\left(1+\phi_{\max } + 2 L \Gamma\right)/d + 1) } + 2\sqrt{\left(C + \Gamma\phi_{\max}\right) /d} \right] .
\end{aligned}
\end{equation*}
The proposition directly follows from \ref{control empirical Rademacher complexity of Gm4} and $R_{n}(\mathcal{G}_{m}^{4})=\mathbf{E}_{\mathcal{S}}\left[\hat{R}_{n}(\mathcal{G}_{m}^{4}, \mathcal{S})\right].$
\end{proof}
